# Supplementary material for: Narrowing down the possible explanations of cosmic acceleration with geometric probes
Source: arXiv:1705.05768 source file (2017-05-16)
Supplement: Supplementary file 1 [file appendix_tables.tex]

\begin{table}
\caption{Precision on the comoving distance from BAO and Weak lensing measurements provided by LSST \citep{2009arXiv0912.0201L}}
\begin{tabular} 
$z$ & Precision \\
\end{tabular}
\end{table}
